# Supplementary material for: Three-wave mixing with three incoming waves: Signal-Idler Coherent Cancellation and Gain Enhancement in a Parametric Amplifier
Source: arXiv:1301.1696 ancillary file (2013-01-08)
Supplement: Supplementary file 1 [file Supplemental_Material.pdf]

# Supplemental material for Three-wave mixing with three incoming waves: Signal-Idler Coherent Cancellation and Gain Enhancement in a Parametric Amplifier

Flavius Schackert,* Ananda Roy, Michael Hatridge, A. Douglas Stone, and Michel H. Devoret
*Departments of Physics and Applied Physics, Yale University, 15 Prospect Street, New Haven, CT 06511*
(Dated: December 9, 2012)

## I. HAMILTONIAN OF JPC

In the rotating-wave approximation (RWA), the working of the JPC can be described by the three-wave mixing Hamiltonian [1]:

$$H^{\mathrm{RWA}} = \hbar\omega_a a^\dagger a + \hbar\omega_b b^\dagger b + \hbar\omega_c c^\dagger c + \hbar g_3 (a^\dagger b^\dagger c + abc^\dagger), \tag{1}$$

where $a, b$ and $c$ represent the resonator modes for the signal, idler and pump respectively with frequencies $\omega_a, \omega_b$ and $\omega_c$ and $g_3$ is the three-wave mixing coefficient.

Assuming a linear coupling between the resonators and the transmission lines carrying waves in and out from them, using input-output theory, we arrive at the equation of motion of the three modes:

$$\begin{aligned}
\frac{da}{dt} &= -i\omega_a a - \frac{\kappa_a}{2} a - i g_3 b^\dagger c + \sqrt{\kappa_a}\tilde{a}^{in}, \\
\frac{db}{dt} &= -i\omega_b b - \frac{\kappa_b}{2} b - i g_3 a^\dagger c + \sqrt{\kappa_b}\tilde{b}^{in}, \\
\frac{dc}{dt} &= -i\omega_c c - \frac{\kappa_c}{2} c - i g_3 ab + \sqrt{\kappa_c}\tilde{c}^{in},
\end{aligned} \tag{2}$$

where the damping coefficients $\kappa_a, \kappa_b$ and $\kappa_c$ are the bandwidths of the modes $a, b, c$ and $\tilde{a}^{in}, \tilde{b}^{in}$ and $\tilde{c}^{in}$ are the input fields that obey the relation $\tilde{a}^{in}(t) = \frac{1}{\sqrt{2\pi}}\int_0^{+\infty} d\omega\ a^{in}[\omega]e^{-i\omega t}$.

## II. UN-DEPLETED PUMP APPROXIMATION

In the un-depleted pump approximation, we assume the pump to be sufficiently intense so that we may neglect the change in its amplitude despite the fact that pump-photons are being converted to signal and idler as a part of the amplification process. Then, we can replace $c$ by its classical average value:

$$c(t) \to \langle c(t)\rangle = \frac{2}{\sqrt{\kappa_c}}\langle c^{in}\rangle, \tag{3}$$

where $\langle c^{in}\rangle = |\langle c^{in}\rangle| e^{-i(\omega_c t + \varphi_p)}$, $\varphi_p$ denoting the pump phase.

Under this approximation, from Eqs. (2),(3) one obtains the scattering matrix for the JPC [1, 2]:

$$\begin{pmatrix} a^{out}[\omega_a] \\ b^{out}[\omega_b]^\dagger \end{pmatrix} = \begin{pmatrix} \sqrt{G_0} & -ie^{-i\varphi_p}\sqrt{G_0 - 1} \\ ie^{i\varphi_p}\sqrt{G_0 - 1} & \sqrt{G_0} \end{pmatrix} \begin{pmatrix} a^{in}[\omega_a] \\ b^{in}[\omega_b]^\dagger \end{pmatrix}, \tag{4}$$

where

$$\sqrt{G_0} = \frac{1 + \rho_0^2}{1 - \rho_0^2}, \quad \rho_0 = \frac{4 g_3 |\langle c^{in}\rangle|}{\sqrt{\kappa_a \kappa_b \kappa_c}}, \tag{5}$$

$G_0$ referred to as the un-depleted gain of the system.

* flavius.schackert@yale.edu

## III. DEPLETED PUMP ANALYSIS

The un-depleted pump approximation works well, as long as the pump strength is much higher than the signal or idler. Assuming equal photon fluxes in the signal and idler[3], as the ratio of the incident signal photons to the incident pump photons increase, the un-depleted pump approximation becomes progressively worse and one needs to incorporate pump depletion in the treatment.

Obviously, one can numerically solve the equations of motion (Eq. (2)), but in order to have a physical understanding of the depletion, we develop a perturbation expansion in terms of the ratio of the photon fluxes in the signal (idler) and pump input. The aforementioned ratio is denoted by $x$, which is defined as: $x = \frac{\dot{n}_S}{\dot{n}_I} \equiv \frac{|a^{in}|^2}{|c^{in}|^2}$.

We start from the un-depleted pump approximation and treat the pump depletion to be small:

$$\langle c\rangle = \frac{2}{\sqrt{\kappa_c}}\langle c^{in}\rangle + \langle\delta c\rangle e^{-i\omega_c t}, \tag{6}$$

$\langle\delta c\rangle$ denotes the amplitude of depletion. It is worthwhile to mention here that we still treat the pump as a classical amplitude (thereby working only with its average value) and incorporate depletion self-consistently.

Inserting Eq. (6) in Eq. (2), we arrive at an equation of motion for $\langle\delta c\rangle$:

$$\frac{d}{dt}\langle\delta c\rangle = -\frac{\kappa_c}{2}\langle\delta c\rangle - ig_3\langle a(t)b(t)e^{i\omega_c t}\rangle. \tag{7}$$

Searching for stationary values of $\langle\delta c\rangle$:

$$\frac{\kappa_c}{2}\langle\delta c\rangle = -ig_3\langle a(0)b(0)\rangle. \tag{8}$$

We calculate depletion in an iterative scheme: at the first step, we evaluate depletion using the un-depleted scattering matrix and include the depletion evaluated to calculate the scattering matrix at the next iteration. Repeating the process, we arrive at the final depletion and gain. The scheme converges fairly quickly as will be described below.

We make the assumption that both the signal and idler frequencies are sufficiently near each other so that the gain of the amplifier does not vary appreciably as a function of frequency. To evaluate $\langle a(0)b(0)\rangle$, we use Fourier transforms and input-output relations given below:

$$a(0) = \frac{1}{\sqrt{2\pi}}\int_{-\infty}^{\infty} d\omega\ a[\omega], \quad b(0) = \frac{1}{\sqrt{2\pi}}\int_{-\infty}^{\infty} d\omega'\ b[\omega'], \tag{9}$$

$$\sqrt{\kappa_a}a[\omega] = a^{in}[\omega] + a^{out}[\omega], \quad \sqrt{\kappa_b}b[\omega'] = b^{in}[\omega'] + b^{out}[\omega']. \tag{10}$$

Using the expressions of $a^{out}[\omega], b^{out}[\omega']$ from the scattering matrix, we arrive at an equation for $\langle a(0)b(0)\rangle$:

$$\langle a(0)b(0)\rangle = \frac{1}{2\pi}\int_{-\infty}^{\infty} d\omega \int_{-\infty}^{\infty} d\omega'\langle a[\omega]b[\omega']\rangle, \tag{11}$$

where

$$\begin{aligned}\sqrt{\kappa_a\kappa_b}\langle a[\omega]b[\omega']\rangle = \Big\langle &\Big\{(1+\sqrt{G})a^{in}[\omega] - ie^{-i\varphi_p}\sqrt{G-1}b^{in}[\omega-\omega_c]\Big\}\\ &\Big\{(1+\sqrt{G})b^{in}[\omega'] - ie^{-i\varphi_p}\sqrt{G-1}a^{in}[\omega'-\omega_c]\Big\}\Big\rangle\end{aligned} \tag{12}$$

The correlation functions in the above equation can be expressed in terms of the spectral densities using the relation:

$$\langle a^{in}[\omega]a^{in}[\omega']\rangle = \mathcal{N}_a^{in}\Big[\frac{\omega-\omega'}{2}\Big]\delta(\omega+\omega'), \tag{13}$$

where neglecting quantum noise for a CW-drive at frequency $\omega_a$:

$$\mathcal{N}_a^{in}[\omega] = 2\pi P_a^{in}[\delta(\omega-\omega_a) + \delta(\omega+\omega_a)], \tag{14}$$

where $P_a^{in}$ is the photon flux of the incoming drive tone at angular frequency $\omega_a$. Assuming a fixed phase relation between the signal and the idler (which we denote by $\phi$) and equal fluxes in the signal and idler port, we arrive at the following expression for $\langle a(0)b(0)\rangle$:

$$\begin{aligned}\Rightarrow \langle a(0)b(0)\rangle = \frac{e^{-i\varphi_p}}{\sqrt{\kappa_a\kappa_b}}P_a^{in}\Big\{&(1+\sqrt{G})^2 e^{i(\phi+\varphi_p)} - 2i(1+\sqrt{G})\sqrt{G-1}\\ &-e^{-i(\phi+\varphi_p)}(G-1)\Big\},\end{aligned} \tag{15}$$

where we have neglected the negative frequency since an equal contribution comes for the pump and is canceled in the definition of $x$. Using the obtained expression for $\langle a(0)b(0)\rangle$ in Eq. (8), we arrive at:

$$\langle \delta c\rangle_n = -i\Big(\frac{2}{\sqrt{\kappa_c}}|\langle c^{in}\rangle|e^{-i\varphi_p}\Big)\frac{\rho_0}{4}x\frac{1}{\sqrt{G_{n-1}}}\Big\{(1+\sqrt{G_{n-1}})^2 e^{i(\phi+\varphi_p)} \\ -2i(1+\sqrt{G_{n-1}})\sqrt{G_{n-1}-1} - e^{-i(\phi+\varphi_p)}(G_{n-1}-1)\Big\} \tag{16}$$

where $\langle \delta c\rangle_n$ is the depletion calculated at the $n^{th}$ iteration, which makes use of the gain computed at the $(n-1)^{th}$ iteration. Thus, the effective pump strength at the $n^{th}$ iteration is:

$$\langle c\rangle_n = e^{-i(\omega_c t+\varphi_p)}\frac{2}{\sqrt{\kappa_c}}|\langle c^{in}\rangle|\Big[1 - i\frac{\rho_0}{4}x\frac{1}{\sqrt{G_{n-1}}}\Big\{(1+\sqrt{G_{n-1}})^2 e^{i(\phi+\varphi_p)} \\ -2i(1+\sqrt{G_{n-1}})\sqrt{G_{n-1}-1} - e^{-i(\phi+\varphi_p)}(G_{n-1}-1)\Big\}\Big], \tag{17}$$

which can be used to calculate the gain at $n^{th}$ iteration using Eq. (5). Taking the limit $n\to\infty$ and dropping the suffix, we arrive at:

$$\rho = \rho_0\Big|\Big[1 - i\frac{\rho_0}{4}x\frac{1}{\sqrt{G}}\Big\{(1+\sqrt{G})^2 e^{i(\phi+\varphi_p)} \\ -2i(1+\sqrt{G})\sqrt{G-1} - e^{-i(\phi+\varphi_p)}(G-1)\Big\}\Big]\Big|, \tag{18}$$

$$\sqrt{G} = \frac{1+\rho^2}{1-\rho^2}. \tag{19}$$

The above equation can be solved self-consistently or iteratively to obtain the gain. As is evident from the expression, the gain is modulated as the phase difference between the signal and idler is varied.

Expanding in powers of $\frac{1}{\sqrt{G}}$, the above expression reduces to:

$$\rho = \rho_0\Big|\Big[1 - \frac{\rho_0}{2}x\Big\{\sqrt{G}\Big(1-\sin(\phi+\varphi_p)\Big) + \Big(1 + i\cos(\phi+\varphi_p) \\ -\sin(\phi+\varphi_p)\Big) + \frac{1}{2\sqrt{G}}\Big(-1+2i\cos(\phi+\varphi_p)\Big)\Big\} + O\Big(\frac{1}{G}\Big)\Big]\Big|, \tag{20}$$

which clearly manifests the phase modulation of gain (set $\phi+\varphi_p=\pi/2$ for gain enhancement, $\phi+\varphi_p=3\pi/2$ for gain depletion).

## IV. BANDWIDTHS AND DETUNINGS IN THE EXPERIMENT

We would like to emphasize the hierarchy of all relevant bandwidths and frequency offsets present in the experiments: The largest bandwidth is the JPC dynamical bandwidth, which is $\geq 1.5$ MHz, followed by the probe tone offset of 100 kHz (still within the JPC dynamical bandwidth). Then comes the spectrum analyzer (SA) resolution bandwidth (RBW) of at least 36 Hz (captures either signal/idler or probe tone power, but never both) and finally the detuning $\delta f = 0.1$ Hz (much smaller than RBW to have enough phase resolution). The chosen RBW's are fast enough to capture the dynamics of the JPC as a function of $\phi$, while being small enough for the experiment to have a sufficient signal-to-noise ratio (SNR), and also making sure not to capture the signal/idler tones when measuring the probe tone power.

---


[1] B. Abdo, A. Kamal, and M. H. Devoret, *Fluctuating Nonlinear Oscillators: From Nanomechanics to Quantum Superconducting Circuits*, edited by M. Dykman (OUP Oxford, 2012) pp. 119–141.

[2] N. Bergeal, R. Vijay, V. E. Manucharyan, I. Siddiqi, R. J. Schoelkopf, S. M. Girvin, and M. H. Devoret, Nat. Phys. **6**, 296 (2010).

[3] The generalization to the unequal case is easily done and provides no additional information.
